# Supplementary material for: Drag Reduction in Flows Past 2D and 3D Circular Cylinders Through Deep Reinforcement Learning
Source: arXiv:2309.02109 source file (2023-09-05)
Supplement: Supplementary file 1 [file appendix.tex]

\newpage
\appendix
\section*{Appendix: Effect of the Actuators}
 In order to compute the total thrust contribution to the force from the actuators, we express the force acting on the fluid passing through the actuators with Newton's second law

 \begin{equation} \label{eq:thrust01}
    \mathbf{F}=\frac{d}{dt}(m \mathbf{V}) = \sum_{i=0}^{N_a-1} \dot{m}_i |\mathbf{V}_i| \mathbf{n}_i \,,
 \end{equation}

 where $\dot{m}_i$ is the mass flux through actuator $i$, $\mathbf{V}_i$ is the constant mean fluid velocity and $\mathbf{n}_i = (\cos \theta_i, \sin \theta_i, 0)$ is the outward facing normal vector to the cylinder surface. Since we are only interested in thrust created through fluid ejection, we do not include pressure contributions.

 The mass flux can be computed from

 \begin{equation}\label{eq:thrust02}
 \dot{m}_i = \int_{-L/2}^{L/2} \int_{\theta_i-\theta_a/2}^{\theta_i+\theta_a/2} \rho v^r_i(\theta) R \; \mathrm{d} \theta \mathrm{d}z\,,
 \end{equation}

 where $L$ and $R$ is the cylinder length and radius, $\theta_a$ is the angle that corresponds to the arc length of each actuator, $\theta_i$ is the angle where each actuator is centered, $\rho$ is the fluid density, $v^r_i$ is the radial fluid velocity, given from~\cref{eq:action} and $\theta$ is the polar angle. By using~\cref{eq:thrust02} and~\cref{eq:action}, we get

 \begin{equation}\label{eq:thrust04}
 \dot{m}_i = \frac{2c\rho LRU  a_i\theta_a}{\pi}\,,
 \end{equation}

where the time index $t$ was omitted. The mean velocity is, by definition

 \begin{equation}\label{eq:thrust05}
 |\mathbf{V}_i| = \frac{\dot{m}_i}{\rho \theta_a R L} = \frac{2 c U| a_i |}{\pi}
 \end{equation}

 Therefore, 
 the thrust force is
 \begin{equation}\label{eq:thrust06}
 F_x = \frac{4c^2 \rho \theta_a LR U^2}{\pi^2} \sum_{i=0}^{N_a-1} (a_i - \bar a)|a_i - \bar a|\cos \theta_i \,,
 \end{equation}
 and 
 the thrust coefficient is 

 \begin{equation}\label{eq:thrust07}
 C_T = \frac{F_x}{\frac{1}{2} \rho U^2 2RL} = \frac{4c^2 \theta_a}{\pi^2} \sum_{i=0}^{N_a-1} a_i|a_i |\cos \theta_i \,.
 \end{equation}

 In the present case $\theta_a = 8^o$ which, along with the other values used, gives us

 \begin{equation}\label{eq:thrust08}
 C_T(a_0,\dots, a_7) = \frac{1}{90 \pi}\sum_{i=0}^{7} a_i|a_i|\cos \theta_i \,.
 \end{equation}

 \Cref{eq:thrust08} expresses the thrust coefficient generated by our actuators as a function of eight variables, the RL actions taken. A numerical maximization of this function results in a maximum value of about $0.018$. As can be seen in~\cref{tab:summary-2d}, at Re=4000, the mean drag coefficient is $1.75$. This means that the thrust force implied by the actuation can only account for a drag reduction of about $1\%$.
